# Supplementary material for: Efficient Quantum Simulation of Open Quantum System Dynamics on Noisy Quantum Computers
Source: arXiv:2106.12882 source file (2021-09-10)
Supplement: Supplementary file 1 [file si.pdf]

# Supplementary Information:
# Efficient Quantum Simulation of Open Quantum System Dynamics on Noisy Quantum Computers

Shin Sun, Li-Chai Shih, and Yuan-Chung Cheng*
*Department of Chemistry, National Taiwan University, Taipei City 106, Taiwan*

## CONTENTS

S1. Single qubit dynamics under $(X)^2$ gates 2
S2. State purity changes under $(X)^2$ gates 3
S3. Single qubit Bloch sphere dynamics under $(X)^2$ gates 4
S4. Noise decomposition and simulation of $(X)^2$ gates 6
S5. Compensating pulse sequence design–$(XZ)^2$ gates and $(XZXZZ)^2$ gates 8
S6. Variance of depolarizing rates of $(X)^2$ gates and $(XZXZZ)^2$ gates 12

## List of Figures

Fig. S1. Single qubit dynamics for the $(X)^2$ gates 2
Fig. S2. Single qubit purity changes for the $(X)^2$ gate 3
Fig. S3. Bloch sphere dynamics generated by applying the $(X)^2$ gate 5
Fig. S4. Fitting of the Bloch sphere dynamics for the $(X)^2$ gate 7
Fig. S5. Illustration of the compensating pulse sequences design 8
Fig. S6. Bloch sphere dynamics for the $(Z)^2$ gate 9
Fig. S7. Bloch sphere dynamics for the $(XZ)^2$ gate 10
Fig. S8. Bloch sphere dynamics for the $(XZXZZ)^2$ gate 11
Fig. S9. Depolarization rates of $(XZXZZ)^2$ and $(X)^2$ on different devices and time 12

## S1. Single qubit dynamics under $(\mathbf{X})^2$ gates

To investigate the qubit dynamics induced by $(X)^2$ gates, we initialized a single qubit in the $|0\rangle$ state and applied multiple $(X)^2$ gates on it. Projective measurement in the computational basis is then performed to obtain the population in $|0\rangle$ $(P_0)$ as a function of the number of $(X)^2$ gates applied. Figure S1 shows population in $|0\rangle$ as a function of the number of $(X)^2$ gates applied. We performed the same experiment on different days as well as different qubits on the IBM-Q quantum computer. Note that $(X)^2$ gate corresponds to the identity operation. However, in all cases, the $P_0$ quickly decreases, and the dynamics behave as highly-noisy fluctuations tending towards the maximally disordered state $(P_0 = 0.5)$. We speculated that the dynamics can be explained by two predominant types of errors in the X gates. An over-rotation of the X gates results in the population change at the initial stages, and decoherent-type error dominates at large number of X gates, which in turn drives the population towards 0.5. We thus perform further state characterization to assess the dynamics of the noises induced by $(X)^2$ gates (Secs. S2-S4). Furthermore, the population dynamics under different parameters behaves very differently even qualitatively, which also signify the highly unstable nature of the $(X)^2$ gate noises.

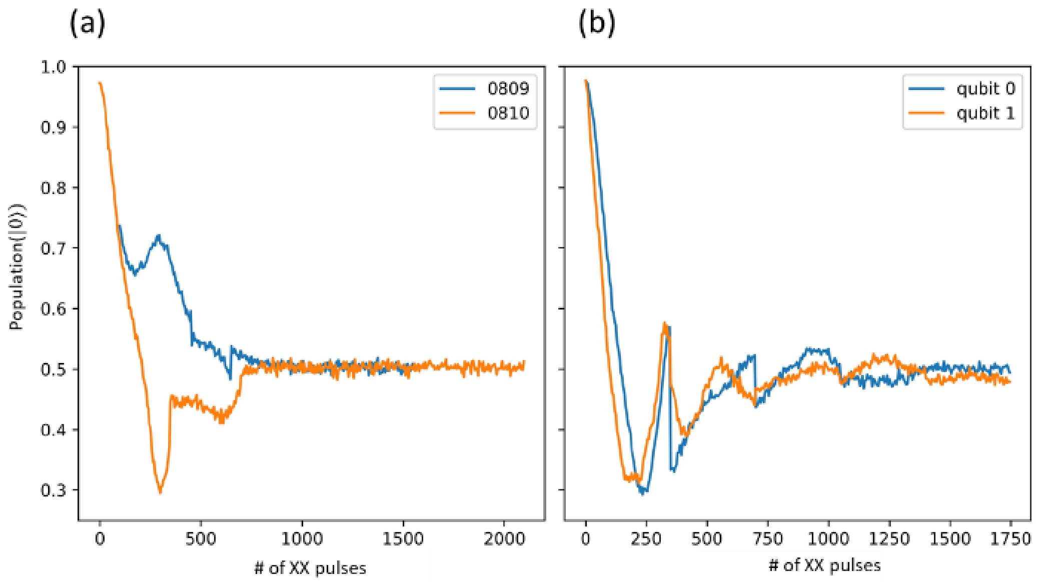


FIG. S1. **Single qubit dynamics for the $(\mathbf{X})^2$ gates.** Populations of $|0\rangle$ as functions of the number of applied $(X)^2$ gates are plotted. (a) Results on different days (8/9 and 8/10) but on the same physical qubit. (b) Results on different physical qubits. All experiments were performed on ibmq_ourense

## S2. State purity changes under $(X)^2$ gates

To obtain quantitative information about the qubit coherence under $(X)^2$ gates, we initialize the qubit in four states ($|0\rangle, |1\rangle, |+\rangle = (|0\rangle + |1\rangle)/\sqrt{2}$, $|-\rangle = (|0\rangle + i|1\rangle)/\sqrt{2}$), apply a number of $(X)^2$ gates and measure the expectation values in the Pauli basis. Quantum state tomography is then performed to reconstruct the density matrices (2.1) at each number of $(X)^2$ gates applied. We compute the purity $\gamma \equiv \mathrm{tr}(\rho^2)$ of the states to assess the coherence of qubit under $(X)^2$ gates. Figure S2 shows the purities as functions of the number of $(X)^2$ gates for each input state. The purities generally decrease as the increasing number of $(X)^2$ gates, but the decaying rates are different for each initial state, suggesting that the decoherence errors are state-dependent. The purity information thus provides a direct evidence of the decoherence error introduced by the $(X)^2$ gates.

$$\rho = \frac{I + \mathrm{tr}(\rho\sigma_x)\sigma_x + \mathrm{tr}(\rho\sigma_y)\sigma_y + \mathrm{tr}(\rho\sigma_z)\sigma_z}{2} \tag{2.1}$$

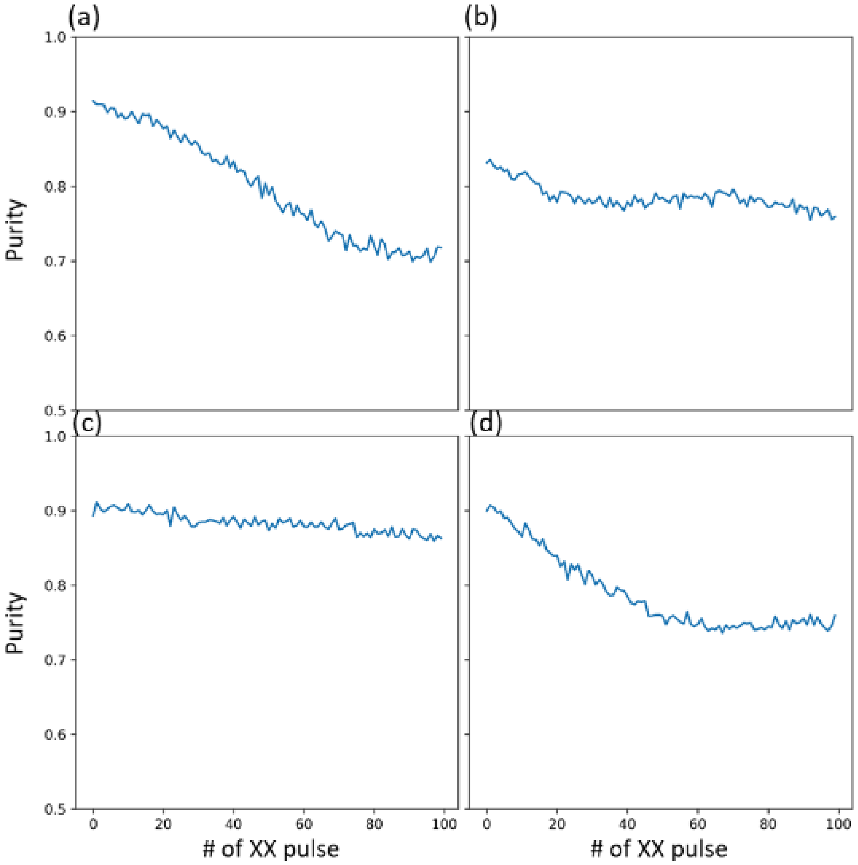


FIG. S2. **Single qubit purity changes for the $(\mathbf{X})^2$ gate.** The state purity as functions of the number of applied $(X)^2$ gates is plotted. (a) – (d) corresponds to initial state = $|0\rangle, |1\rangle, |+\rangle, |-\rangle$, respectively. All experiments were performed on ibmq_bogota.

## S3. Single qubit Bloch sphere dynamics under $(X)^2$ gates

Here we visualize the noise induced by $(X)^2$ gates by plotting the single qubit dynamics as a function of the number of $(X)^2$ applied. We performed quantum state tomography to obtain the quantum states for four different input state ($|0\rangle$, $|1\rangle$, $|+\rangle$, $|-\rangle$). By decomposing the single qubit density matrix with respect to Pauli basis (3.1), we can obtain the Bloch vector representation $(r_x, r_y, r_z)$ of the qubit state.

$$\rho = \frac{I + r_x\sigma_x + r_y\sigma_y + r_z\sigma_z}{2} \tag{3.1}$$

Because we perform the input-output analysis in a tomographically-complete bases, the procedure is also equivalent to quantum process tomography, and it provides an intuitive understanding about the underlying qubit dynamics when presented on a Bloch sphere. Figure S3 shows the $(X)^2$ dynamics for different initial states. The Bloch vector for the single qubit state is represented by a dot, and the dot is traced continuously with increasing number of $(X)^2$ gates. For each input state, the dynamics could be seen as rotations around the X axis (arising from the over-rotation of X gates), plus an uniform contraction towards the center (typical behavior for the depolarizing noises). It is worth noting that for the initial state $|+\rangle$, being the eigenstate of the X-rotation, shows only contraction.

.

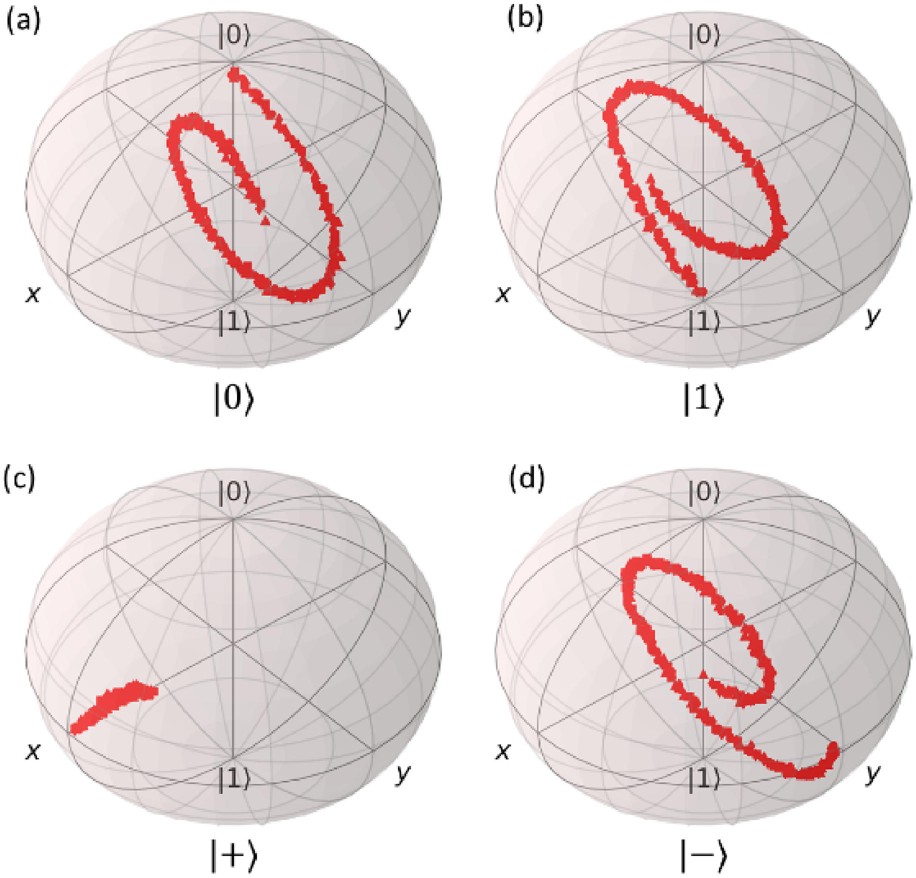


FIG. S3. **Bloch sphere dynamics generated by applying the $(\mathbf{X})^2$ gate.** We initialize the qubit in different initial states, $|0\rangle, |1\rangle, |+\rangle, |-\rangle$, and apply $(\mathrm{X})^2$ gates from 0~300 times to analyze the dynamics. The Bloch vector for the single qubit state is represented by a dot, and the dot is traced continuously with increasing number of $(\mathrm{X})^2$ gates. (a)-(d) all show the effect of rotating around the X axis and shortening towards the center. All experiments were performed on ibmq_manhattan.

# S4. Noise decomposition and simulation of $(X)^2$ gates

To quantitatively analyze the qubit dynamics generated by the $(X)^2$ gate , we build simple mathematical models to describe them. As in Sec. 3 suggests, the quantum process could be seen as a combination of systematic coherent rotation together with depolarization error. In the following experiments, we thus use operator sum representation (4.1) to numerically propagate the qubit states and fit the dynamics obtained (with initial state $=|0\rangle$) in Sec.3 on IBMQ.

$$E(\rho) = \sum_k E_k \rho E_k^\dagger \tag{4.1}$$

where $E_k$ are operation elements, satisfying $\sum_k E_k E_k^\dagger = I$.

We took both coherent rotation (4.2) and depolarization (4.3) into account in our model (The free parameters are rotation angle step $\theta$ and depolarizing probability p).

$$E_0 = e^{-\frac{i\theta X}{2}} = \cos\frac{\theta}{2} I - i\sin\frac{\theta}{2} X = \begin{bmatrix} \cos\frac{\theta}{2} & -i\sin\frac{\theta}{2} X \\ -i\sin\frac{\theta}{2} X & \cos\frac{\theta}{2} \end{bmatrix} \tag{4.2}$$

$$E_1 = \sqrt{1-\frac{3p}{4}}\begin{bmatrix} 1 & 0 \\ 0 & 1 \end{bmatrix},\ E_2 = \sqrt{\frac{p}{4}}\begin{bmatrix} 1 & 0 \\ 0 & 1 \end{bmatrix},\ E_3 = \sqrt{\frac{p}{4}}\begin{bmatrix} 1 & -i \\ i & 1 \end{bmatrix}, E_4 = \sqrt{\frac{p}{4}}\begin{bmatrix} 1 & 0 \\ 0 & -1 \end{bmatrix} \tag{4.3}$$

In Fig. S4, we plot both the Bloch sphere dynamics for the $(X)^2$ gates (red dots), and the fitted dynamics (green). It can be noted that the parameters suitable for the (a) case, cannot reproduce the dynamics for other states (b-d) well for long time. This suggests the state-dependent nature of the quantum gate noises, and could be investigated in the future.

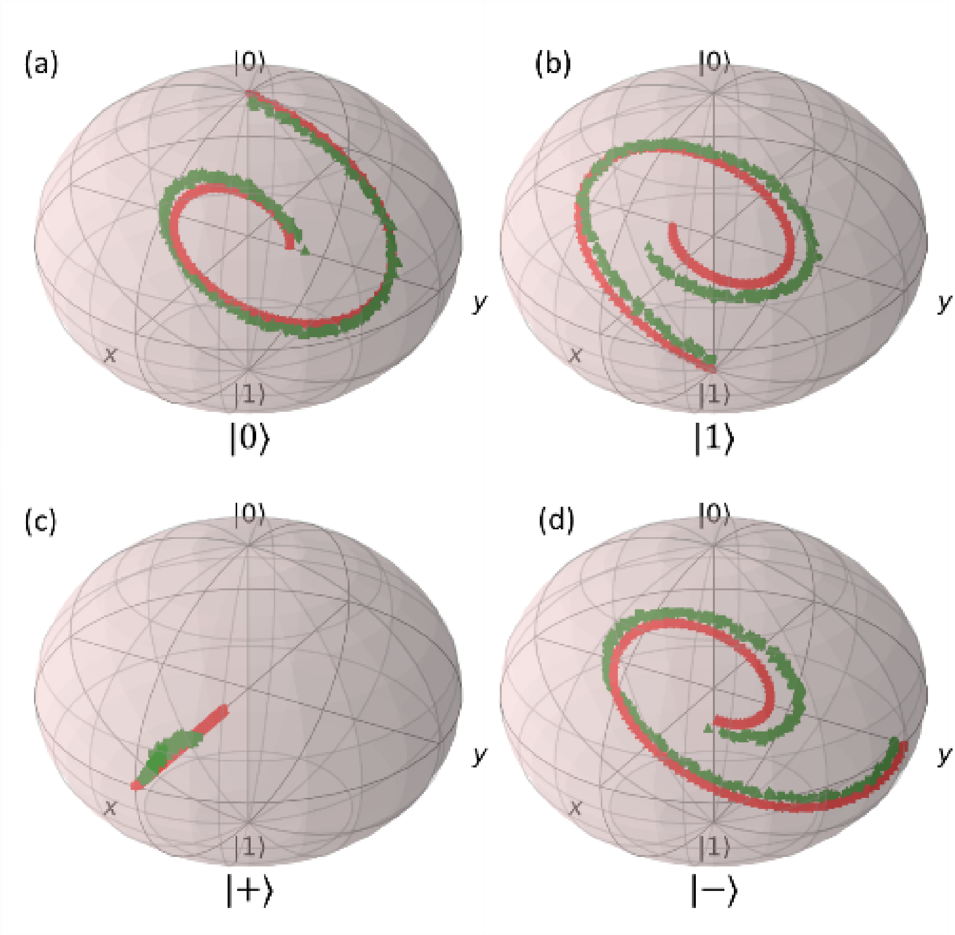


FIG. S4. **Fitting of the Bloch sphere dynamics for the $(X)^2$ gate.**
The Bloch sphere dynamics for the $(X)^2$ gate (red) in Fig. S3 are fitted with qubit dynamics with rotation angle step $\theta = 0.013$ and depolarization probability $p = 0.005$.

**S5. Compensating pulse sequence design – $(XZ)^2$, $(XZXZZ)^2$ gates**

In order to adaptively eliminate the over-rotation in the $(X)^2$ gate without knowing the over-rotation angle in advance, we resort to the echo-type techniques to correct the coherent error (Fig. S5). We first assess the Bloch sphere dynamics of multiple Z gates (Fig. S6) to make sure they do not introduce excess error by themselves.

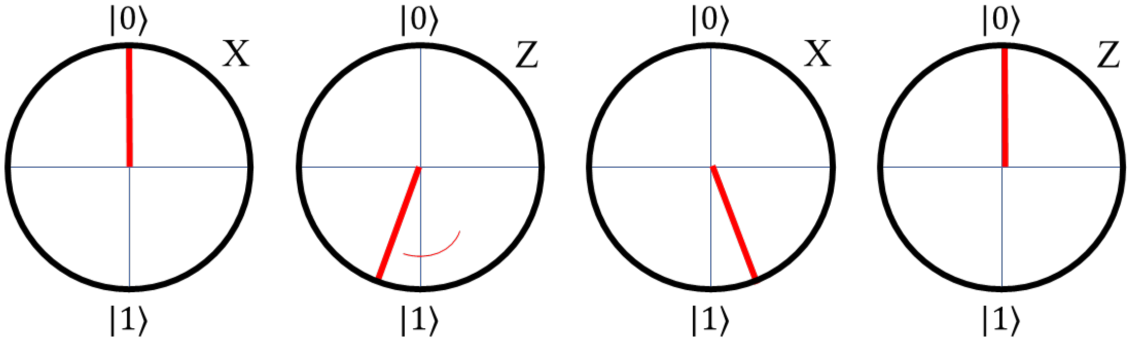


FIG. S5. **Illustration of the compensating pulse sequences design.** The circle is a projection of the Bloch sphere on YZ-plane. To dynamically correct the over-rotation error, first, a X gate is applied. The over-rotation is then turned into an under-rotation by applying a phase (Z) gate. The over-rotation of the second applying X gates then cancels the under-rotation. Finally, another Z gate is applied to recover identity.

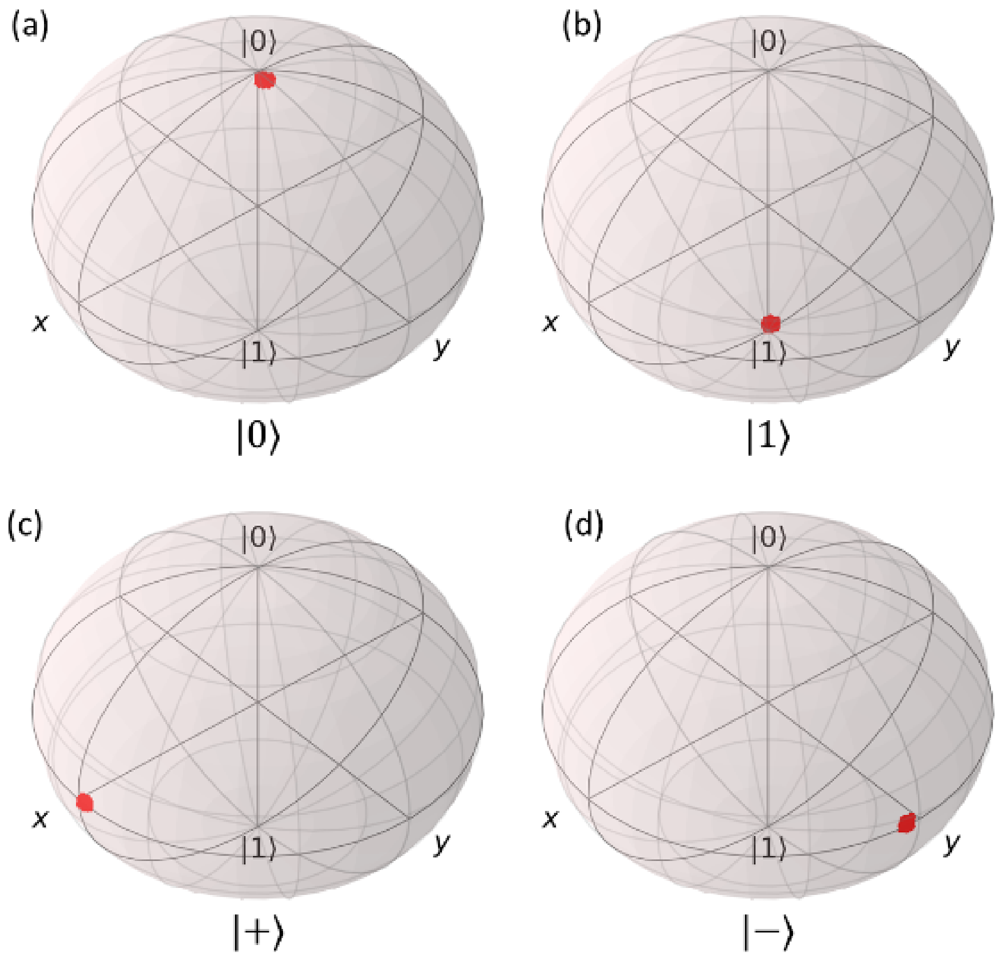


FIG. S6. **Bloch sphere dynamics for the $(\mathbf{Z})^{\mathbf{2}}$ gate.** We initialize the qubit in four basis state, and apply $(Z)^2$ gates from 0~100 times to analyze their behaviors. Each point on the Bloch Sphere represent the density matrix at each number of applied $(Z)^2$gates. Experiments were performed on ibmq_paris.

We then assess the dynamics of $(XZ)^2$ gates by following the same procedure as in Sec. S3. The results are again plotted in Fig. S7. For the input states $|0\rangle$ (Fig. S7 (a)), the dynamics still contain a systematic rotation part. We proposed that this is due to the phase error in the Z gates, which still causes systematic rotations. Therefore, we chose to compensate the systematic rotation again by adopting the $(XZXZZ)^2$ gates.

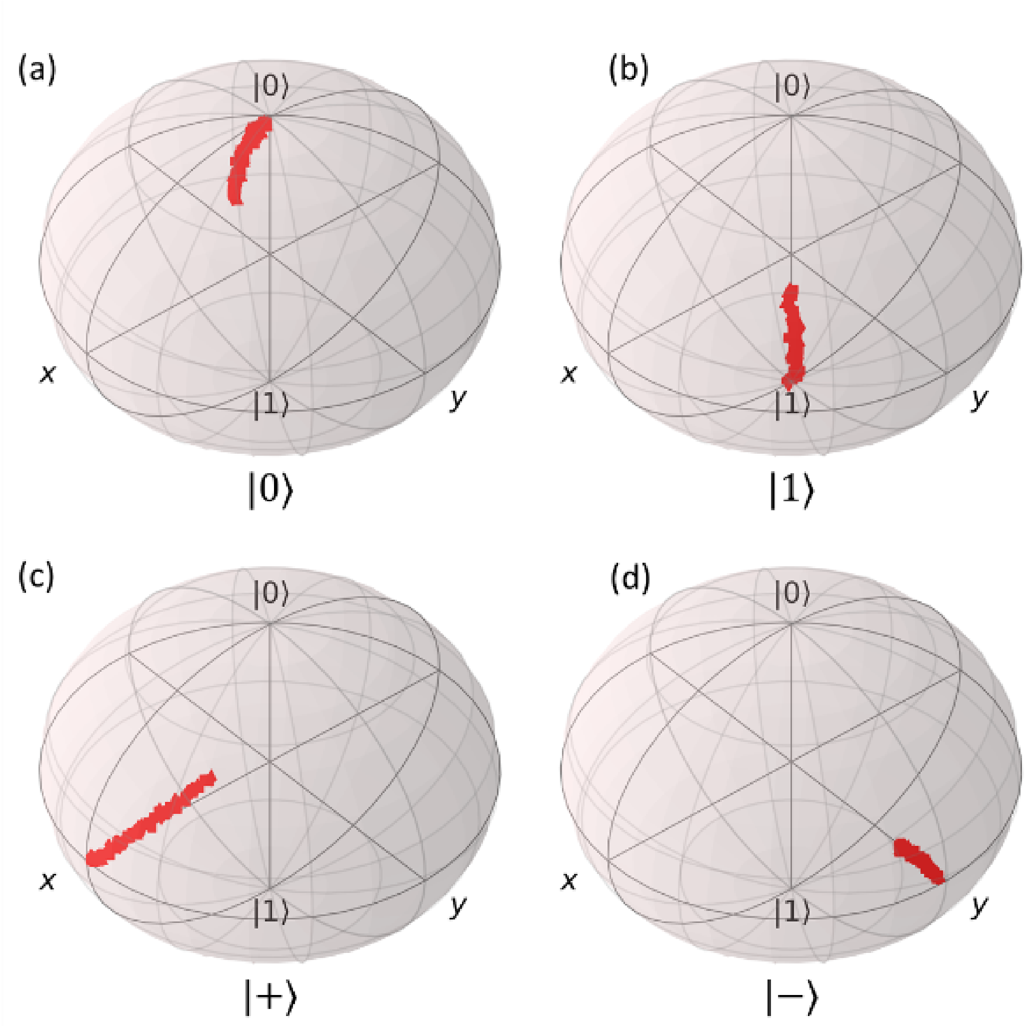


FIG. S7. **Bloch sphere dynamics for the $(\mathbf{XZ})^2$ gate.** We initialize the qubit in four basis state, and apply $(XZ)^2$ gates from 0~100 times to analyze their behaviors. Each point on the Bloch Sphere represent the density matrix at each number of applied $(XZ)^2$gates. In the case of (a) , a systematic rotation is still present. Experiments were performed on ibmq_paris.

Furthermore, in the case of $(XZXZZ)^2$, it can be seen from the Bloch sphere dynamics (Fig. S8) that for all input states, the systematic rotation in the dynamics is much eliminated. Thus, the $(XZXZZ)^2$ can be regarded as good decoherence-inducing gate for our purpose to introduce dissipation into the model system in the main text.

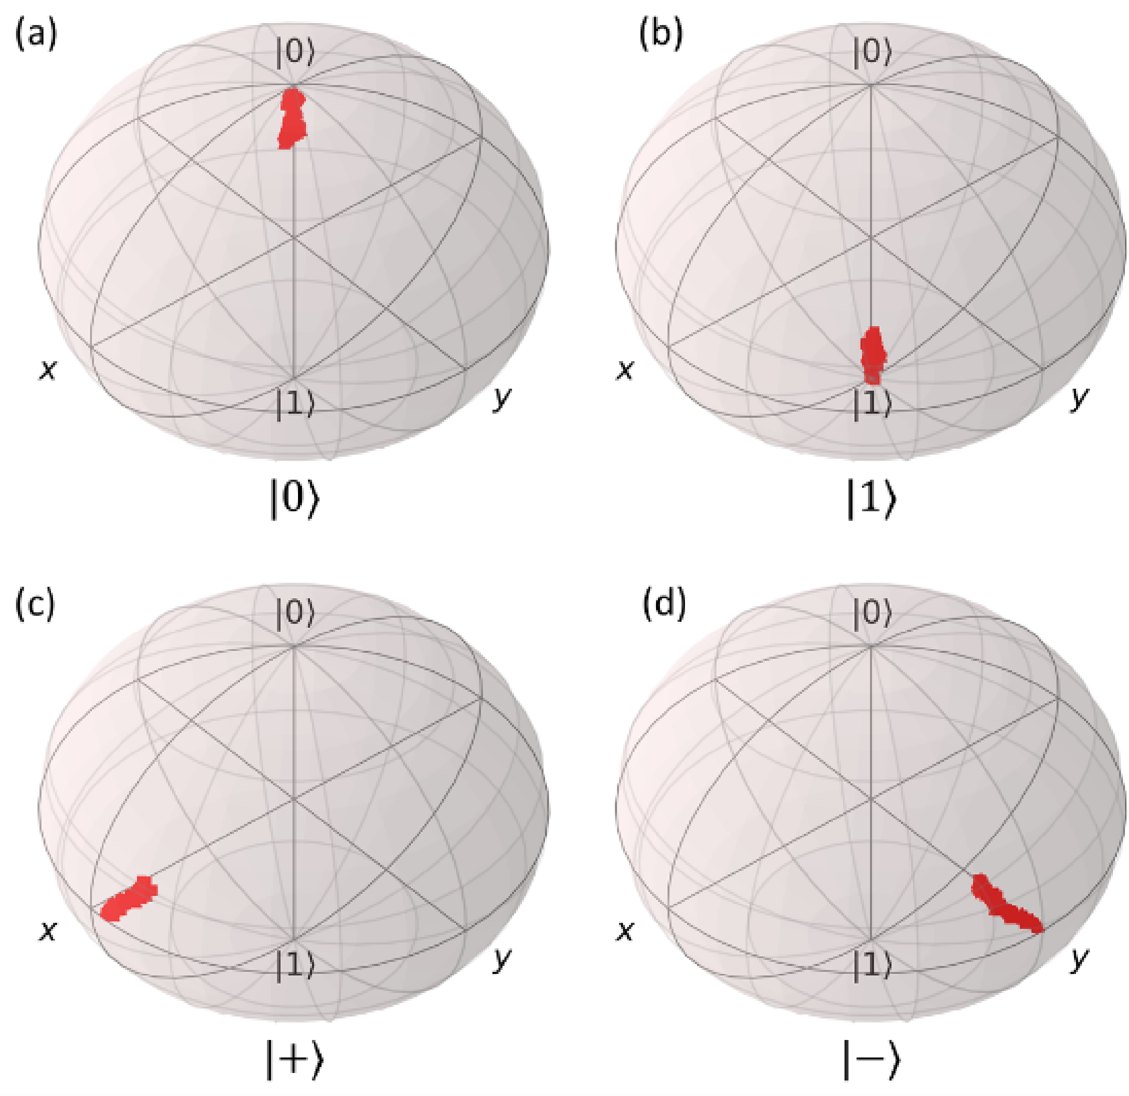


FIG. S8. **Bloch sphere dynamics for the $(\mathbf{XZXZZ})^2$ gate.** We initialize the qubit in four basis state, and apply $(XZXZZ)^2$ gates from 0~100 times to analyze their behaviors. Each point on the Bloch Sphere represent the density matrix at each number of applied $(XZ)^2$gates. Experiments were performed on ibmq_manhattan.

## S6. **Variance of depolarizing rates of $(XZXZZ)^2$ and $(X)^2$**

Here we assess the fluctuation of the decoherence noise strengths for the single-qubit decohernece-inducing gates. To this end, we perform state tomography to obtain single qubit Bloch sphere dynamics under $(XZXZZ)^2$ and $(X)^2$ gate sequences, and fit the dynamics with our model as in Sec.4. We then extract the depolarization rate and assess their behaviors on different devices and days (Fig. S9). Three consecutive experiments were performed and fitted independently to support a statistical analysis. For the $(XZXZZ)^2$ case, the depolarization rate shows a consistent trend among devices (Fastest: Manhattan, Slowest: Bogota). In the case of manhattan, the depolarization rate exhibited large fluctuations, and are not significantly different across days. In the case of paris and bogota, the deviation of noises was much smaller, suggesting the stability of the noises under $(XZXZZ)^2$ were better than manhatten. Except on 12/27, the depolarization rates on three devices were all quantitively different than others. As for the case of $(X)^2$ gates, the depolarization rates were all smaller than that of $(XZXZZ)^2$ due to a smaller number of pulses per identity, and the stabilities were also better in general.

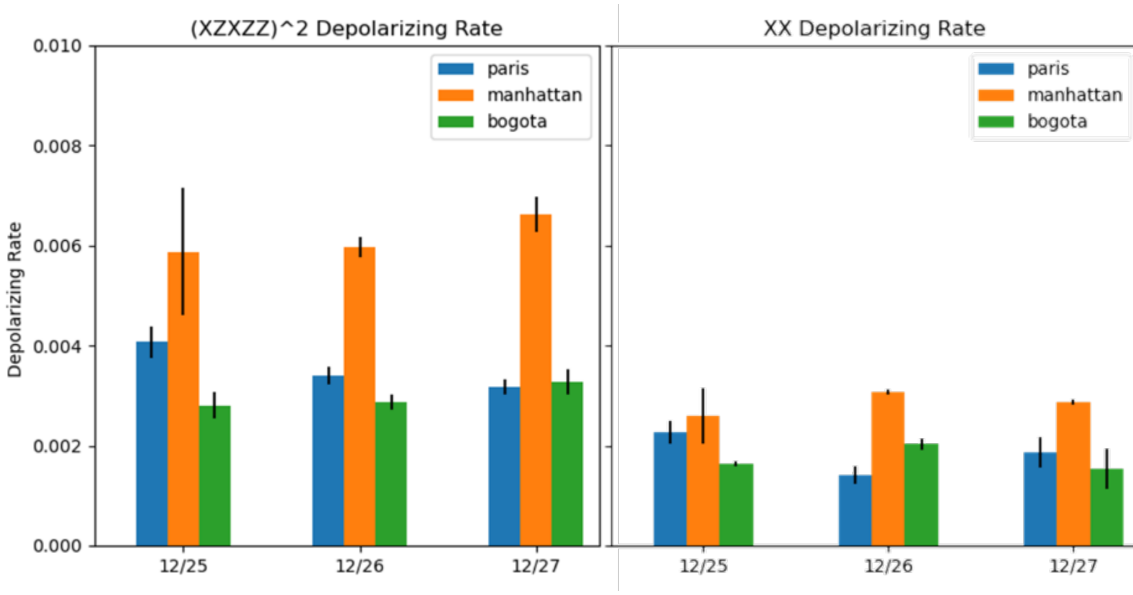


FIG. S9. **Depolarization rates of $(XZXZZ)^2$ and $(X)^2$ on different devices and time.** The fitted depolarization rates for the $(XZXZZ)^2$ and $(X)^2$ gates on different devices and days are shown. The error bars are calculated from three consecutive experiments.
